# Supplementary material for: NVIDIA Spectrum-X: Hardware-Accelerated Multiplane Networking for Large-Scale AI Training
Source: arXiv:2605.21187 source file (2026-10-20)
Supplement: Supplementary file 1 [file multiplane_asymmetry_setup.tex]

\section{Multiplane load balancing setup}
\label{appendix:multiplane_lb_setup}

\cref{fig:mp-asymmetry-setup} illustrates the setup for \cref{ssec:multiplane_lb}. 

\input{figures/mp_asymmetry_setup}
